# Supplementary material for: On Overcoming Miscalibrated Conversational Priors in LLM-based Chatbots
Source: arXiv:2406.01633 source file (2024-06-01)
Supplement: Supplementary file 1 [file notation.tex]

\section{Notation}
\label{sec:notation}
In Table \ref{tab:notation}, we present an overview of the notation used in the paper.
\begin{table}[!htb]
{%
	\caption{Notation used in our paper, with notes on interpretation.} \label{tab:notation}
	\resizebox{\textwidth}{!}{\begin{tabular}{|lll|}
	\hline 
        % Queries, copilot responses, and associated attributes
        \multicolumn{3}{|l|}{\textbf{Queries, copilot responses, and associated attributes} explanation here} \\ \hline
        \multicolumn{1}{|l|}{Fully-specified query} 
            & \multicolumn{1}{l|}{
            $\begin{aligned}
            q_f \in Q
            \end{aligned}$}
            &  test\\ \hline
        \multicolumn{1}{|l|}{Partially-specified/masked query}
            & \multicolumn{1}{l|}{
            $\begin{aligned}
            q_m \in Q
            \end{aligned}$}
            &  test\\ \hline
        \multicolumn{1}{|l|}{Copilot response strategy}             
        & \multicolumn{1}{l|}{
            $\begin{aligned}
            \pi: Q \rightarrow Y
            \end{aligned}$}
            &  test\\ \hline
        \multicolumn{1}{|l|}{Copilot response (given $q, \pi$)}
        & \multicolumn{1}{l|}{
            $\begin{aligned}
            y \in Y \ | \ q \in Q, \pi \in \Pi
            \end{aligned}$}
            &  test\\ \hline
        \multicolumn{1}{|l|}{Minimum viable copilot response}
        & \multicolumn{1}{l|}{
            $\begin{aligned}
            
            \end{aligned}$}
            &  test\\ \hline
        % Synthetic query generation
        \multicolumn{3}{|l|}{\textbf{Synthetic query generation} explanation here} \\ \hline
        \multicolumn{1}{|l|}{Intent space}
        & \multicolumn{1}{l|}{
            $\begin{aligned}
            \mathcal{I}~\coloneq~\{\text{exercise, gift, movie, plant, travel}\}
            \end{aligned}$}
            &  test\\ \hline
        \multicolumn{1}{|l|}{Intent-specific attribute space}
        & \multicolumn{1}{l|}{
            $\begin{aligned}
            \Theta_i \coloneq \{\theta_1, \dots, \theta_{|\Theta_i|}\}
            \end{aligned}$}
            &  test\\ \hline
        \multicolumn{1}{|l|}{Attribute-specific options}
        & \multicolumn{1}{l|}{
            $\begin{aligned}
            X_{\theta \in \Theta_i} \coloneq \{x \ | \ x \text{ is an option for } \theta\}
            \end{aligned}$}
            &  test\\ \hline
        \multicolumn{1}{|l|}{Intent-specific query template}
        & \multicolumn{1}{l|}{
            $\begin{aligned}
            
            \end{aligned}$}
            &  test\\ \hline
        \multicolumn{1}{|l|}{Number of attributes to omit}
        & \multicolumn{1}{l|}{
            $\begin{aligned}
            n \sim U(\{1, \dots, |\Theta_i|\})
            \end{aligned}$}
            &  test\\ \hline
        \multicolumn{1}{|l|}{Masked attributes}
        & \multicolumn{1}{l|}{
            $\begin{aligned}
            \Theta^m_i  \sim U(S_n(\Theta_i))
            \end{aligned}$}
            &  test\\ \hline
        \multicolumn{1}{|l|}{Revealed attributes}
        & \multicolumn{1}{l|}{
            $\begin{aligned}
            \Theta^r_i \coloneq \Theta_i \setminus \Theta^m_i
            \end{aligned}$}
            &  test\\ \hline
        \multicolumn{1}{|l|}{``Depends on'' attributes}
        & \multicolumn{1}{l|}{
            $\begin{aligned}
            
            \end{aligned}$}
            &  test\\ \hline
        % Single-step response evaluation functions
        \multicolumn{3}{|l|}{\textbf{Single-turn response evaluation functions} explanation} \\ \hline
        \multicolumn{1}{|l|}{Utility function}
        & \multicolumn{1}{l|}{
            $\begin{aligned}
            \textbf{utility}_{ST}: (q_m, y_\pi) \in Q \times Y_\pi \mapsto \frac{|\phi(y_\pi)|^\gamma}{|q_{\Theta^m_i}|} \in [0,1]
            \end{aligned}$}
            &  test\\ \hline
        \multicolumn{1}{|l|}{Cost function}
        & \multicolumn{1}{l|}{
            $\begin{aligned}
            
            \end{aligned}$}
            &  test\\ \hline
        \multicolumn{1}{|l|}{Cost-aware utility function}
        & \multicolumn{1}{l|}{
            $\begin{aligned}
            
            \end{aligned}$}
            &  test\\ \hline
        \multicolumn{1}{|l|}{Single-turn oracle policy}
        & \multicolumn{1}{l|}{
            $\begin{aligned}
            
            \end{aligned}$}
            &  test\\ \hline

        % Multi-step response evaluation functions
        \multicolumn{3}{|l|}{\textbf{Multi-turn response evaluation functions} explanation here} \\ \hline
        \multicolumn{1}{|l|}{Utility function}
        & \multicolumn{1}{l|}{
            $\begin{aligned}
            
            \end{aligned}$}
            &  test\\ \hline
        \multicolumn{1}{|l|}{Cost function}
        & \multicolumn{1}{l|}{
            $\begin{aligned}
            
            \end{aligned}$}
            &  test\\ \hline
        \multicolumn{1}{|l|}{Cost-aware utility function}
        & \multicolumn{1}{l|}{
            $\begin{aligned}
            
            \end{aligned}$}
            &  test\\ \hline
        \multicolumn{1}{|l|}{Multi-turn oracle policy}
        & \multicolumn{1}{l|}{
            $\begin{aligned}
            
            \end{aligned}$}
            &  test\\ \hline

	\end{tabular}
 } 
}
\end{table}
